# Supplementary material for: Let Me Do It For You: Towards LLM Empowered Recommendation via Tool Learning
Source: arXiv:2405.15114 source file (2024-05-24)
Supplement: Supplementary file 1 [file 7-Appendix.tex]

\appendix
\section{Representative Failures} \label{sec:appendix}

In this section, we present several representative failure samples from Vicuna and PaLM, categorizing them into three distinct types: (i) Failure to understand the task requirement; (ii) Understanding the task but failing to provide a solution; and (iii) Understanding the task but using incorrect solutions. These cascading failures contribute to the instances where Vicuna and PaLM do not succeed in our task.

\begin{figure}[ht]
\includegraphics[width=0.422\textwidth]{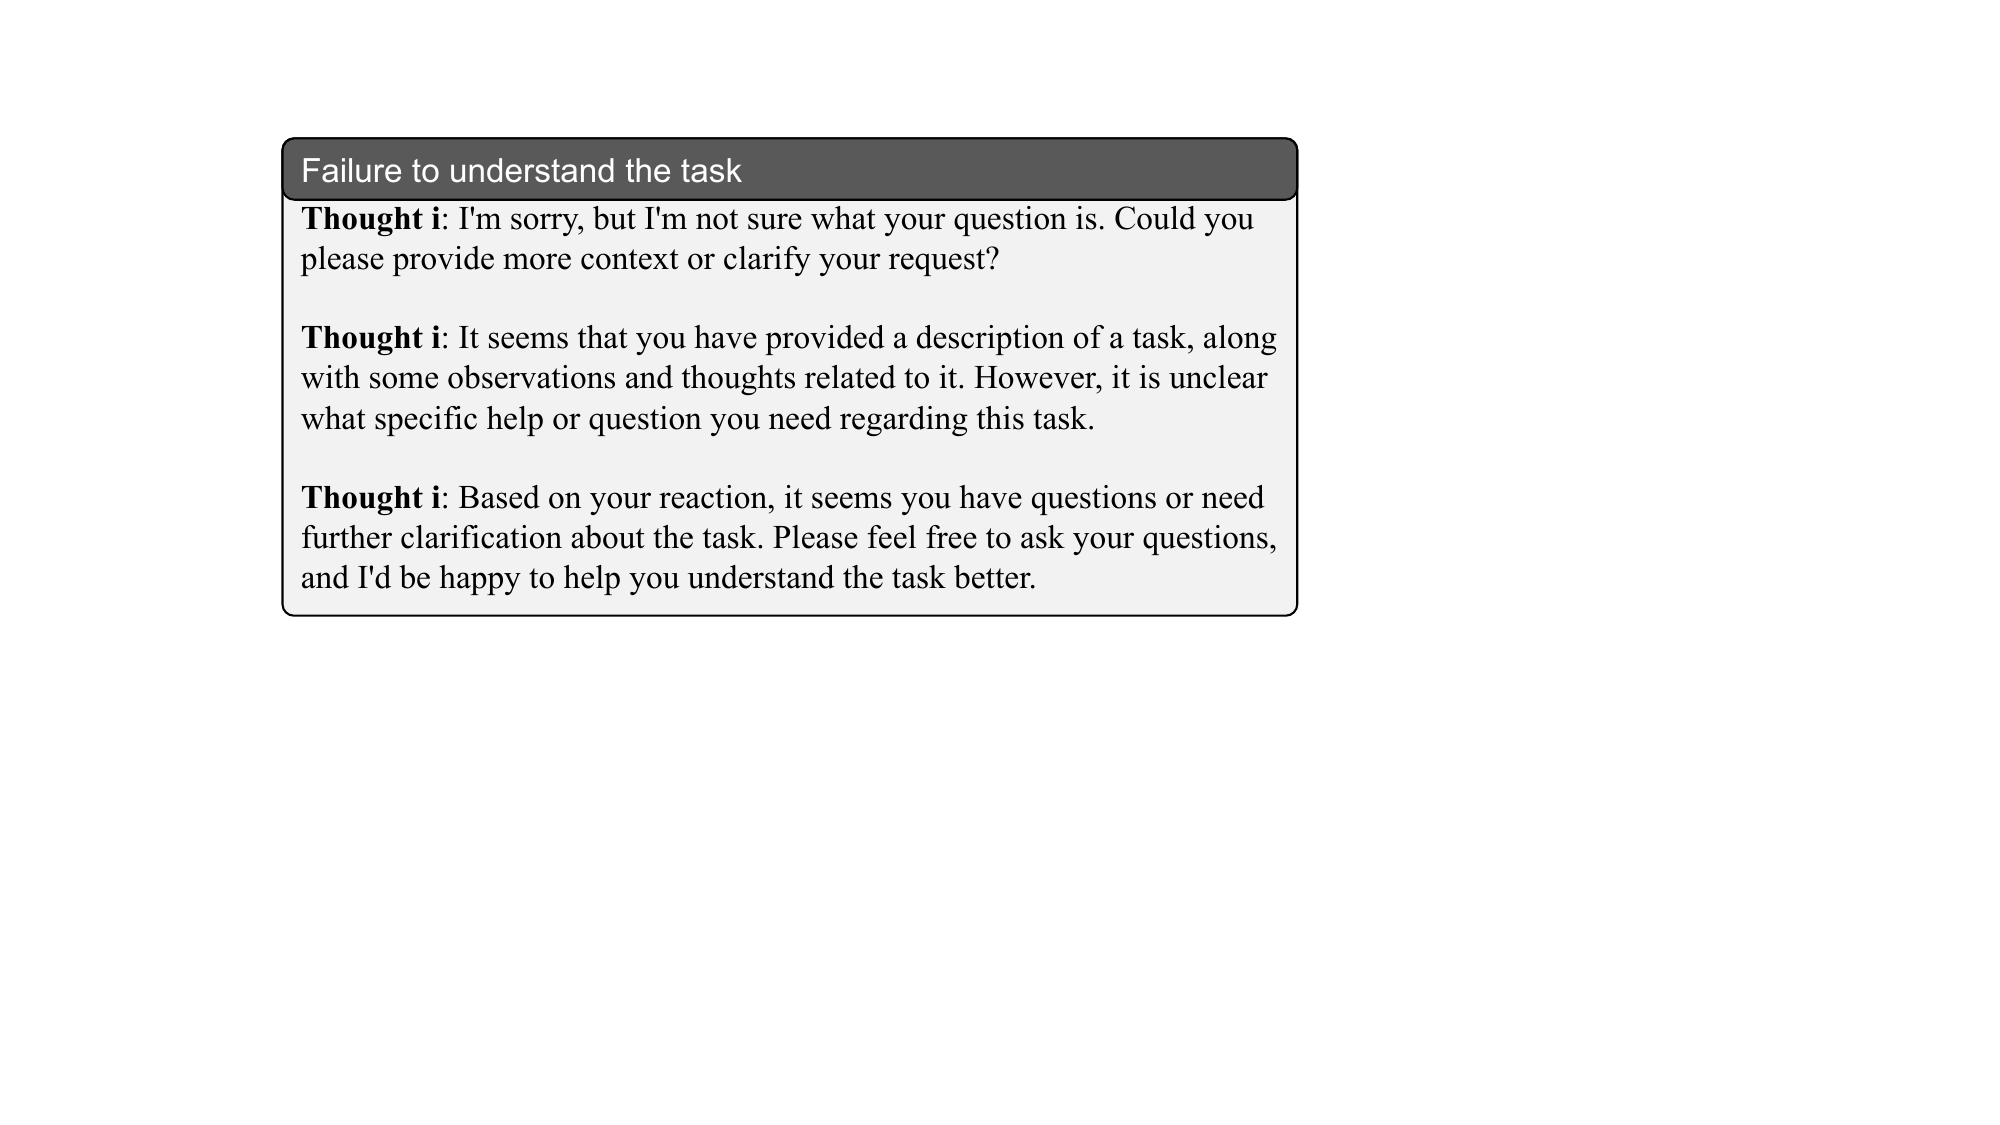}
 \vspace{-10pt}
\label{appd_noques}
\end{figure}

\begin{figure}[ht]
\includegraphics[width=0.422\textwidth]{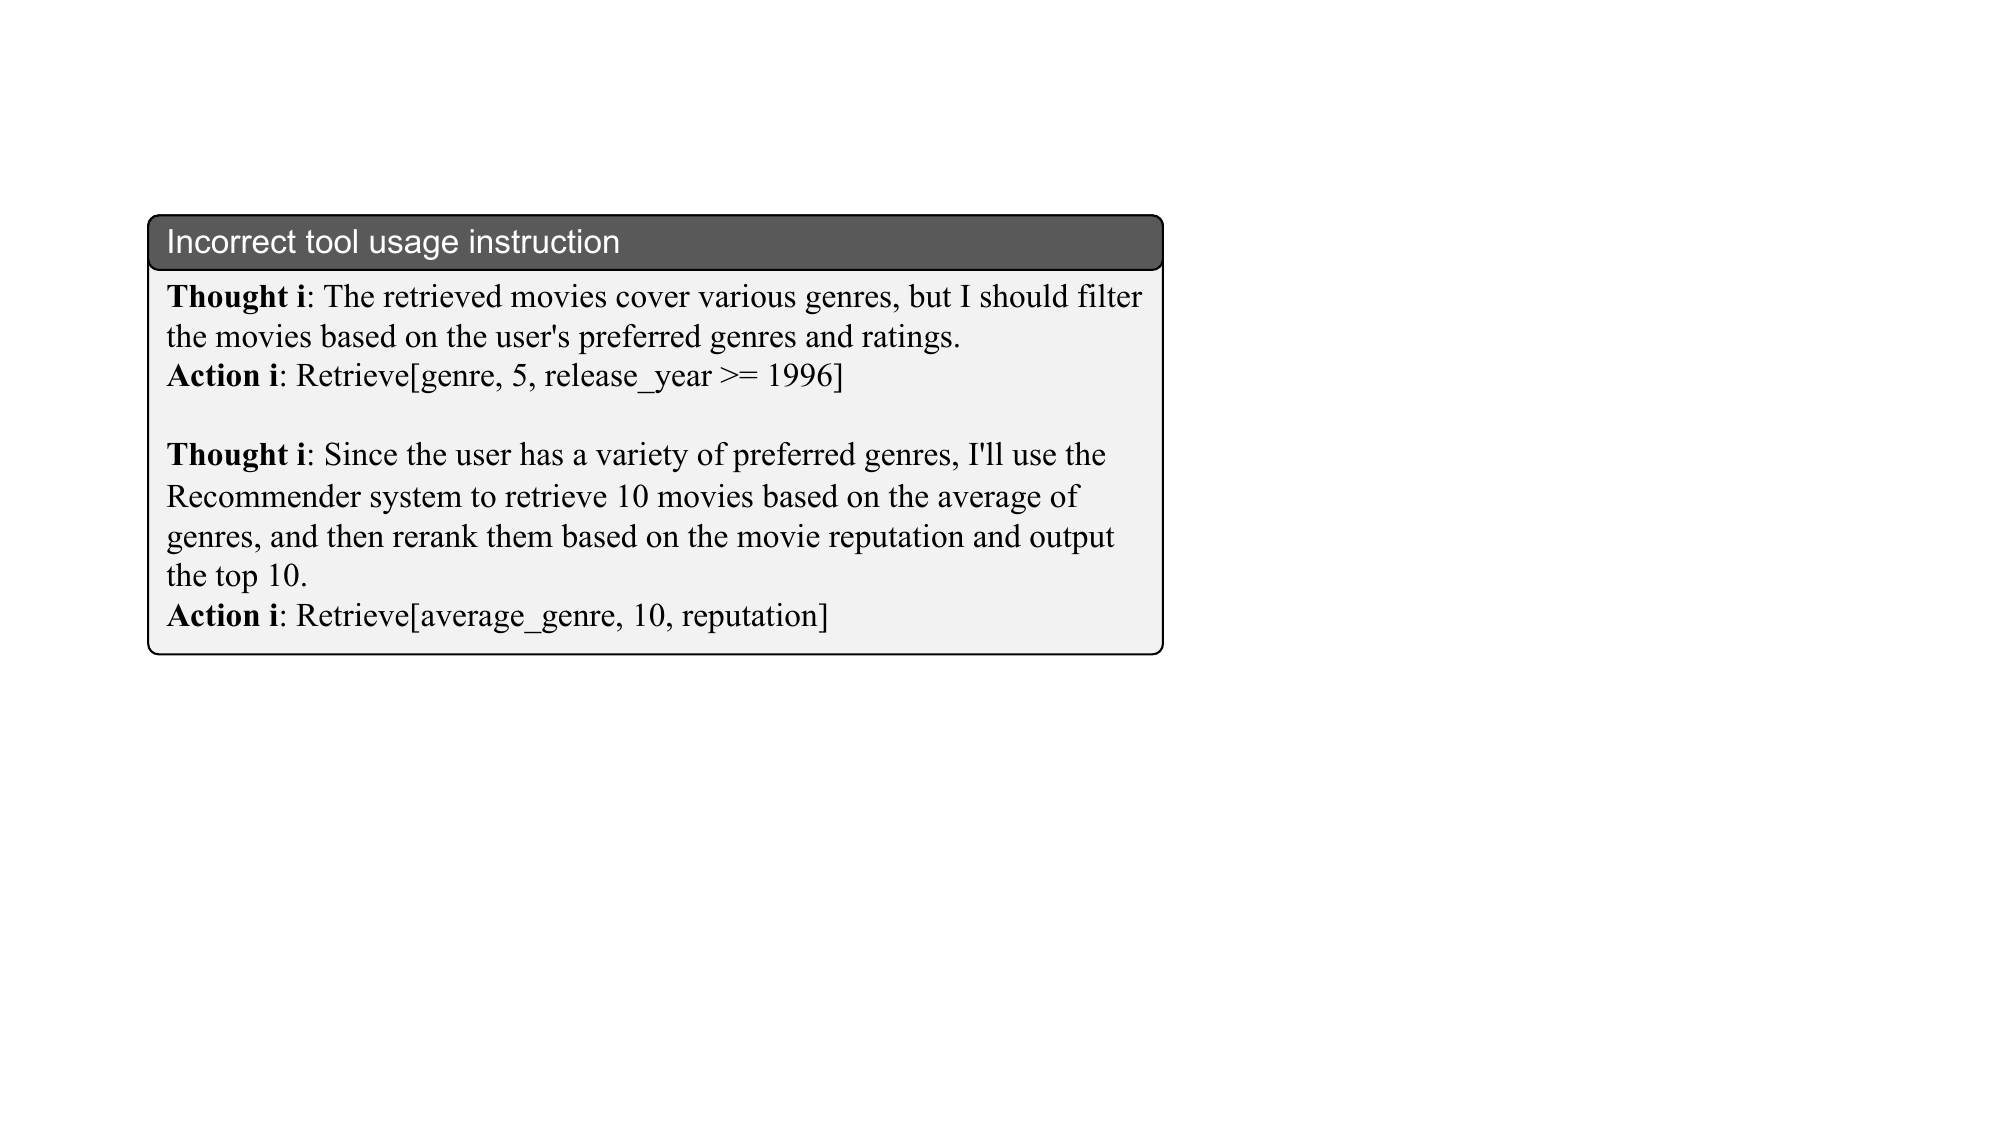}
\vspace{-10pt}
\label{appd_tool}
\end{figure}

\begin{figure}[ht]
\includegraphics[width=0.422\textwidth]{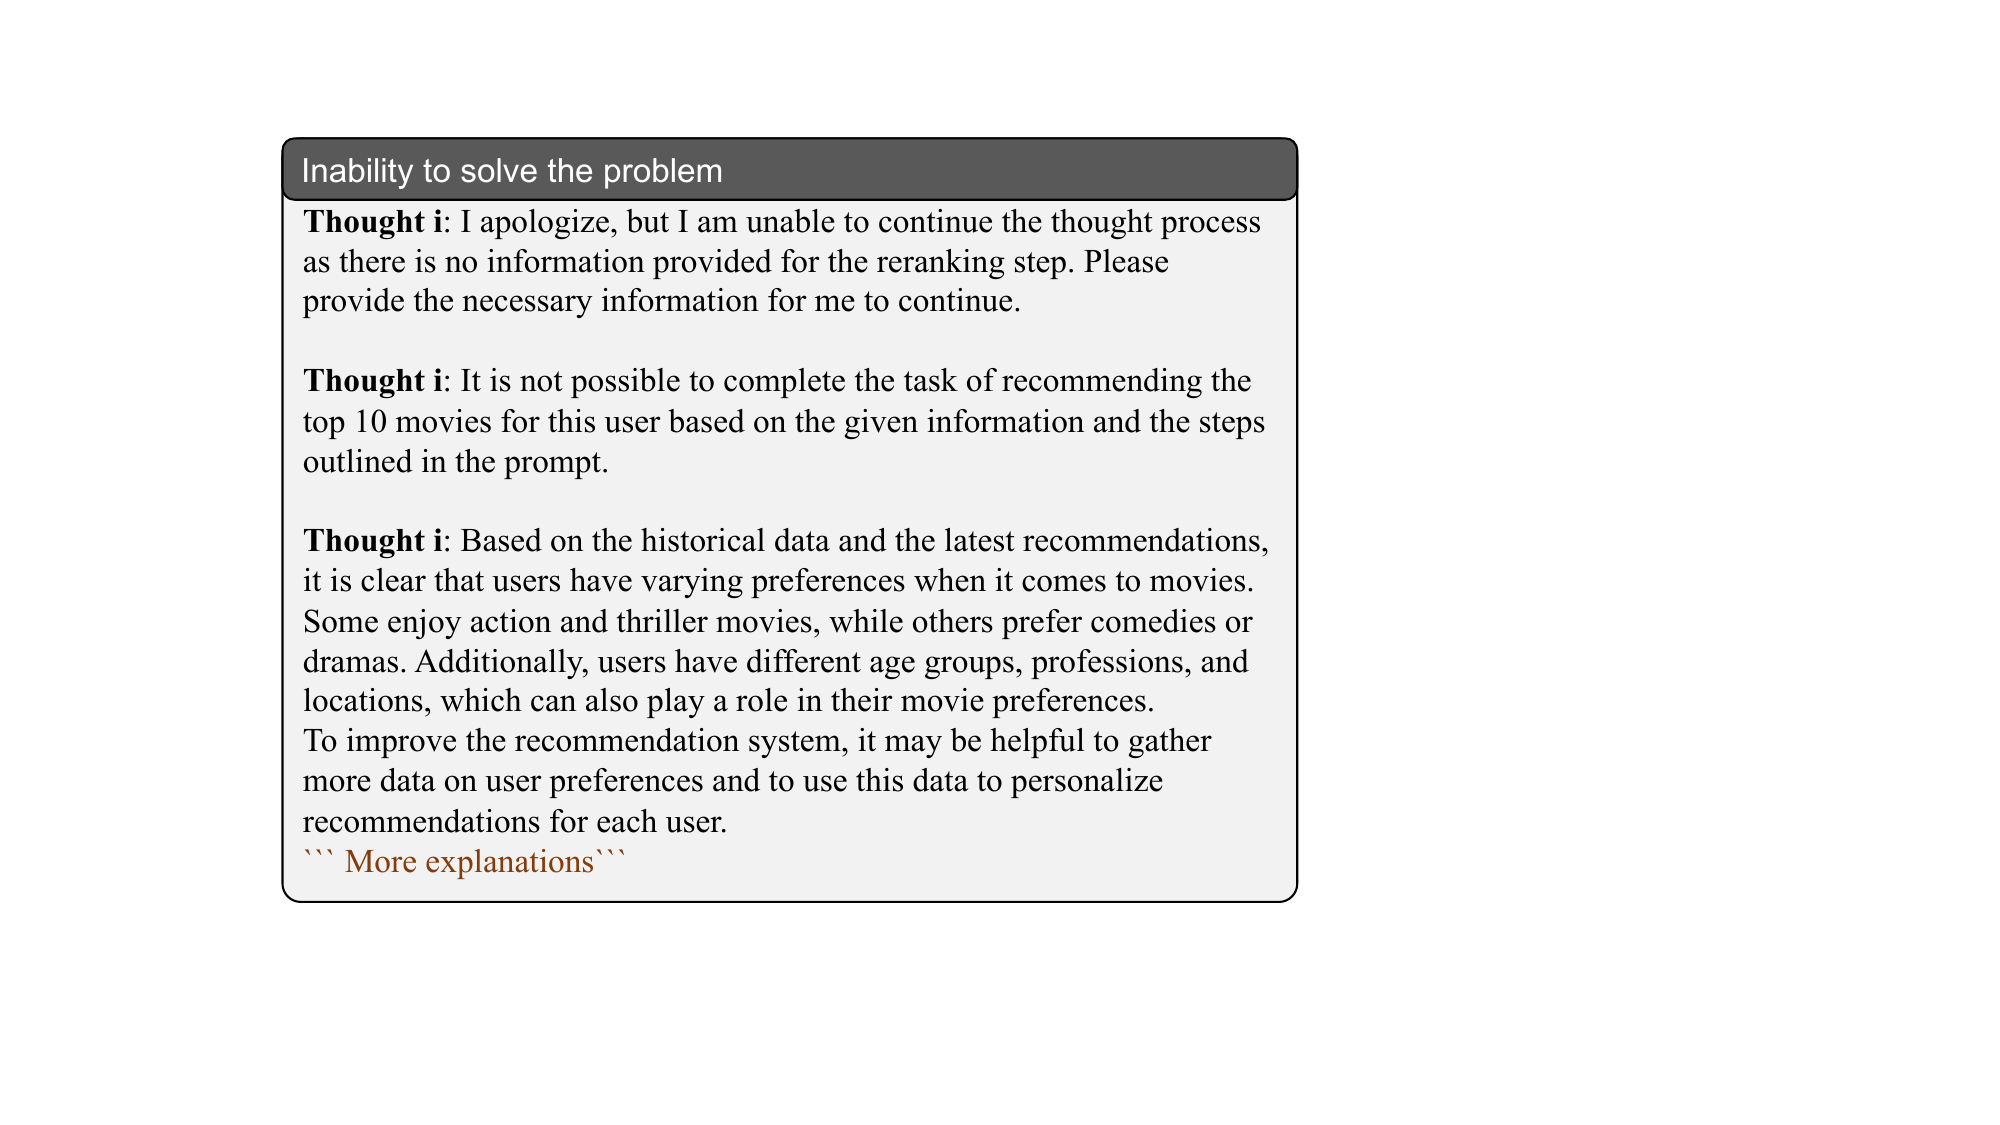}
\label{appd_answer}
\end{figure}
